# Supplementary material for: Open quantum system parameters from molecular dynamics
Source: arXiv:1506.09123 source file (2015-06-30)
Supplement: Supplementary file 1 [file supp_Info_1_6_arXiv.pdf]

# SUPPORTING INFORMATION: Open quantum system parameters from molecular dynamics

Xiaoqing Wang, Gerhard Ritschel, Sebastian Wüster, and Alexander Eisfeld*

*Max-Planck-Institut für Physik komplexer Systeme, Nöthnitzer Str. 38, D-01187 Dresden, Germany*

In this supporting information we provide a comprehensive collection of our various simulation results, and some additional implementation details.

PACS numbers:

## I. TECHNICAL ASPECTS OF MOLECULAR DYNAMICS SIMULATIONS

The structure of Fenna-Matthews-Olson in Chlorobaculum tepidum is obtained from the Protein Data Bank (PDB id 3BSD). The monomer structure with 8 Bacterialchlorophyll a (BChl a) molecules is used. For each BChl a the protonation state of the close histidine is set according to the PKA calculation combined with visual inspection. Histidine 227 and 297 is set as HSE while the other histidine are set as HSD. That means the hydrogen is add on the $\epsilon_2$ nitrogen atom for residue 227 and 297, while hydrogen is add on the $\delta_1$ nitrogen atom for other histidine. All atoms in the protein scaffold, the BChls a and the crystall water molecules are included in the MD simulation. The complex is embedded in a TIP3P water box of dimensions $90 \times 90 \times 90$ Å. Equal amounts of sodium and chloride ions are added to obtain a 0.1 M/L ion concentration.

We have performed the MD simulations using NAMD 2.9. For water molecules, the O-H distance and the H-O-H angle are constrained using the SETTLE algorithm. The Particle Mesh Ewald (PME) method is used for electrostatic summations and periodic boundary conditions are employed. The time step is 1fs.

The system was subjected to energy minimization for 10000 steps using the conjugate gradient algorithm. After minimization the system is heated to the desired temperature $T_0$ by adding 25 K for every 1000 steps and equilibrated with a 500ps simulation using the harmonic constraint on the position of the backbone of protein. The following 10ns equilibration is performed at $T_0$ and 1 atm pressure. We refer to this way of obtaining the initial state for the production runs as method (A).

As discussed in the main text, for 77 K and 200 K we also followed different procedures to obtain a spread of different initial conditions for the production runs. To this end we started from the 300K initial state obtained from method (A). For method (B) we then set the temperatur to the desired lower temperature, where we equilibrate for 10 ns. For method (C) we first set the temperatur to 310K for 500ps and then to the desired lower temperature, where we equilibrate for 10 ns.

*Electronic address: `eisfeld@mpipks-dresden.mpg.de`

## II. ENERGY-GAP TRAJECTORIES

In the main article we show the energy gap trajectories for 300K and 77K for the 'standard' equalibration scheme (A). Here, we also provide for the same equilibration scheme the trajectory for 200K.

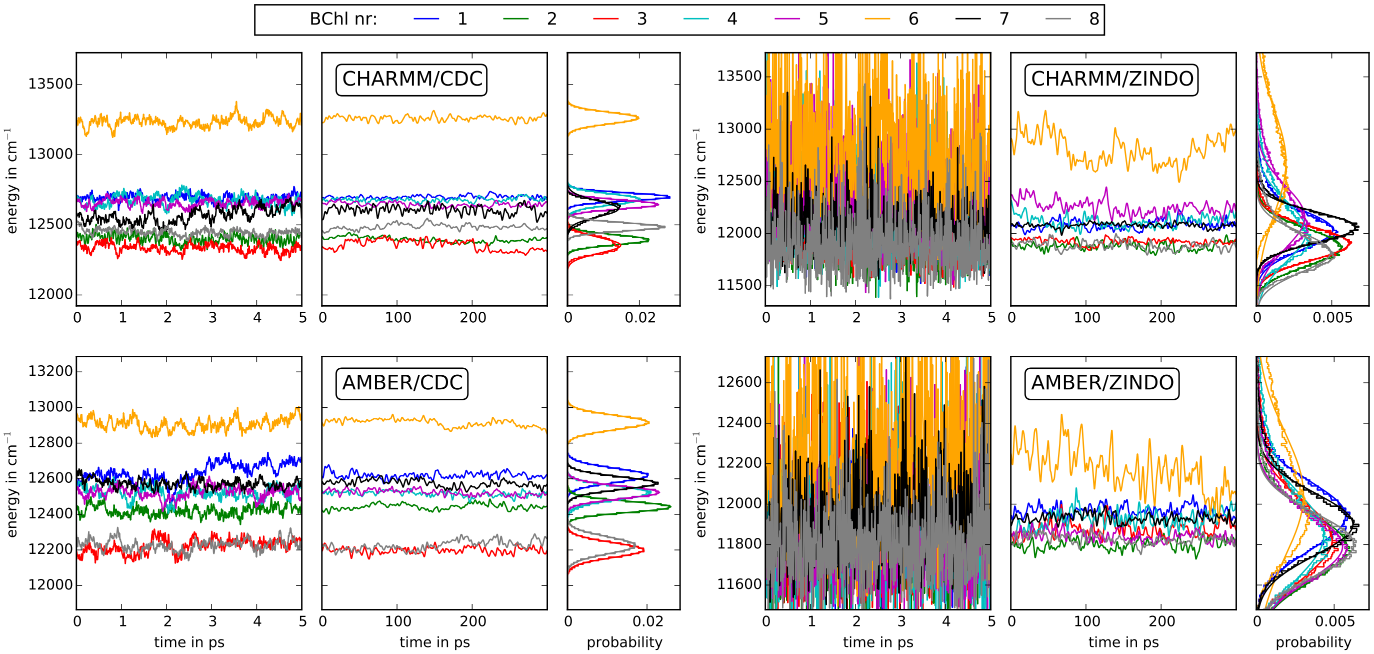


FIG. 1: Same as Fig. 2 of the main article but for 200K.

## III. SITE ENERGIES

Figures 2 and 3 show the mean site energies and the standard deviations of the energy gap distributions for the CDC and the ZINDO calculations, respectively.

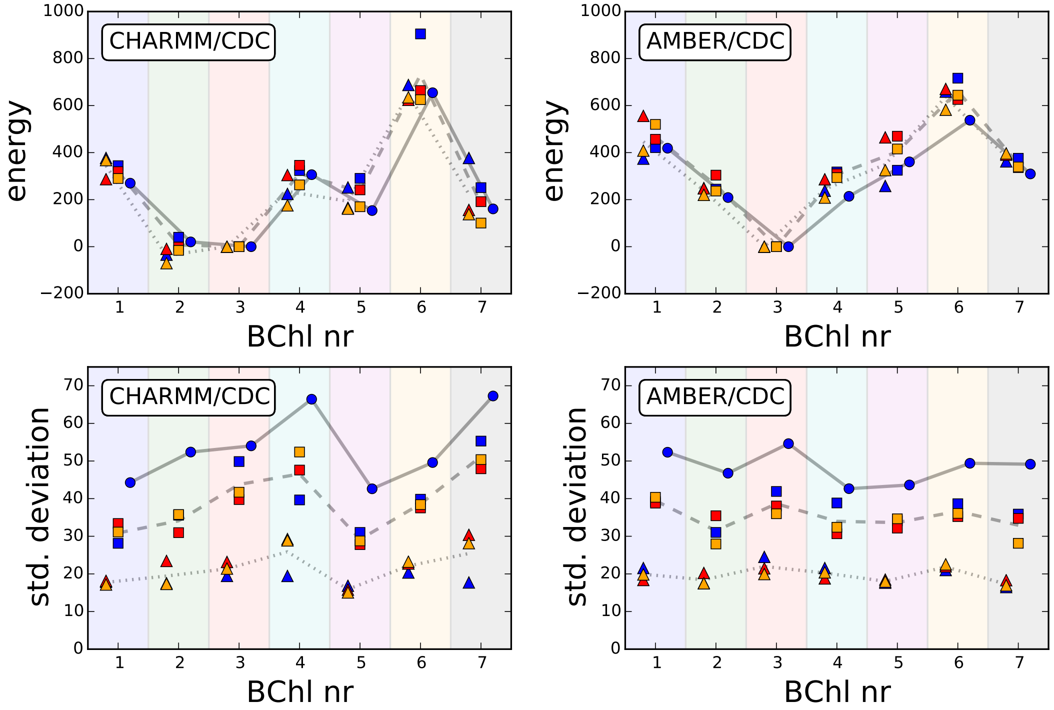


FIG. 2: Mean site energies (upper row) and standard deviations (lower row) of the energy-gap distributions obtained from CDC simulations at 77K (triangles), 200K (squares) and 300K (circ) for the two different force fields. Left column: CHARMM, right column: AMBER. The colors denote the different initial conditions (blue: A, red: B, orange: C).

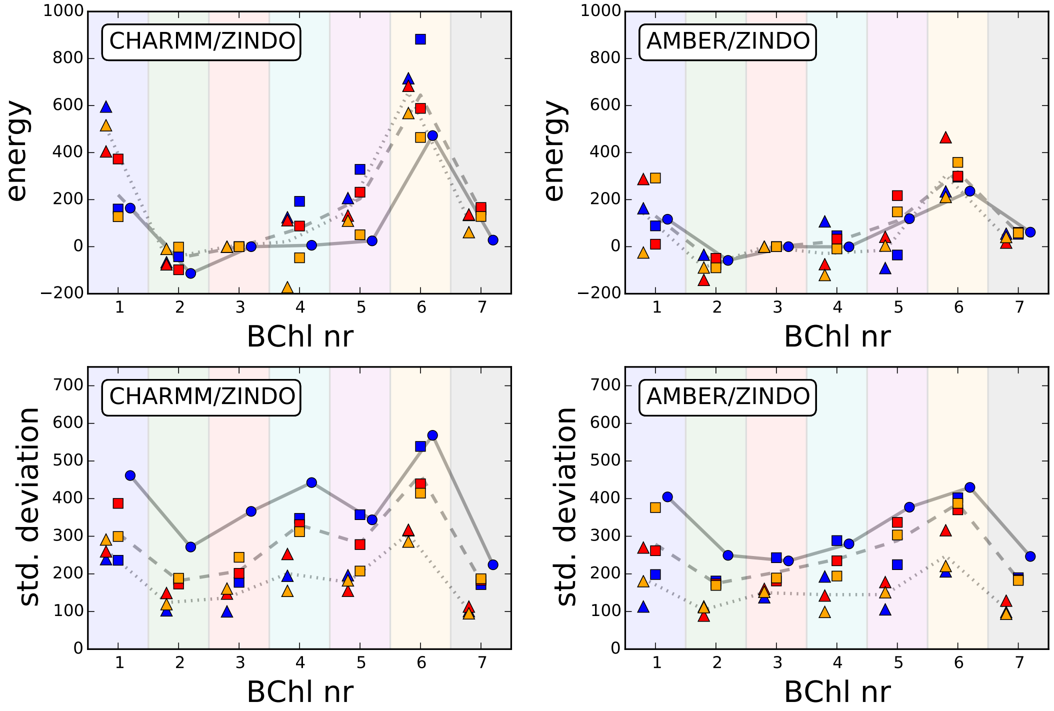


FIG. 3: Same as Fig. 2 but for the ZINDO calculations. Note the different scales of the standard deviation compared to the CDC results.

## IV. CORRELATION BETWEEN THE ENERGY GAPS AT DIFFERENT BCHLS

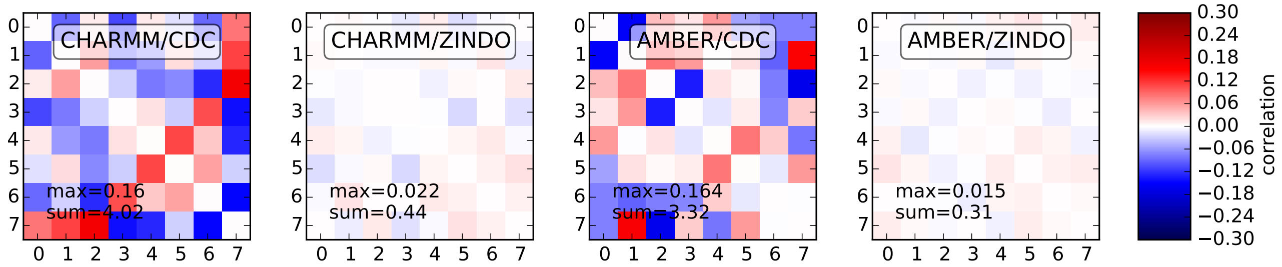


FIG. 4: Correlations between the energy gap fluctuations at different sites at $T = 300K$.

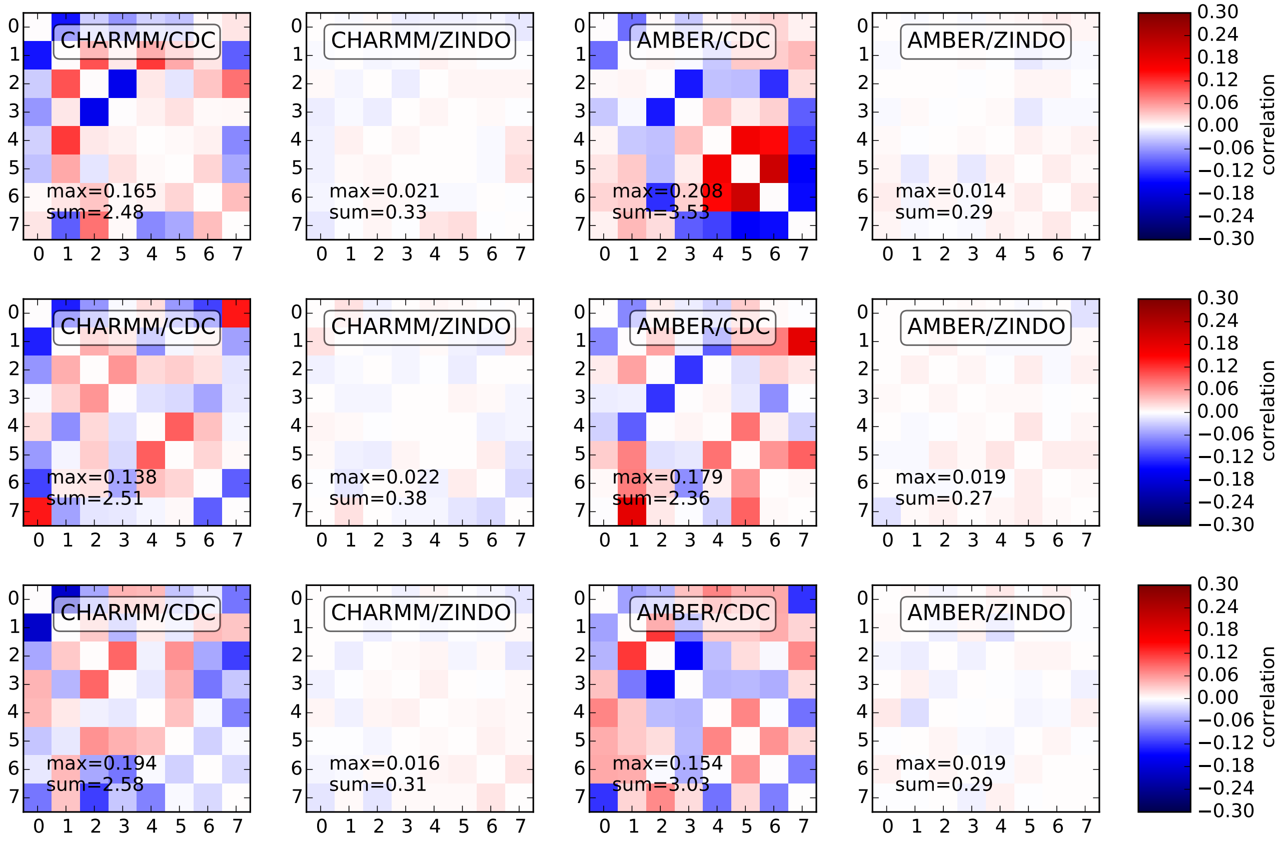


FIG. 5: Correlations between the energy gap fluctuations at different sites at $T = 200K$. From top to bottom: initial condition according to equilibration scheme A, B and C.

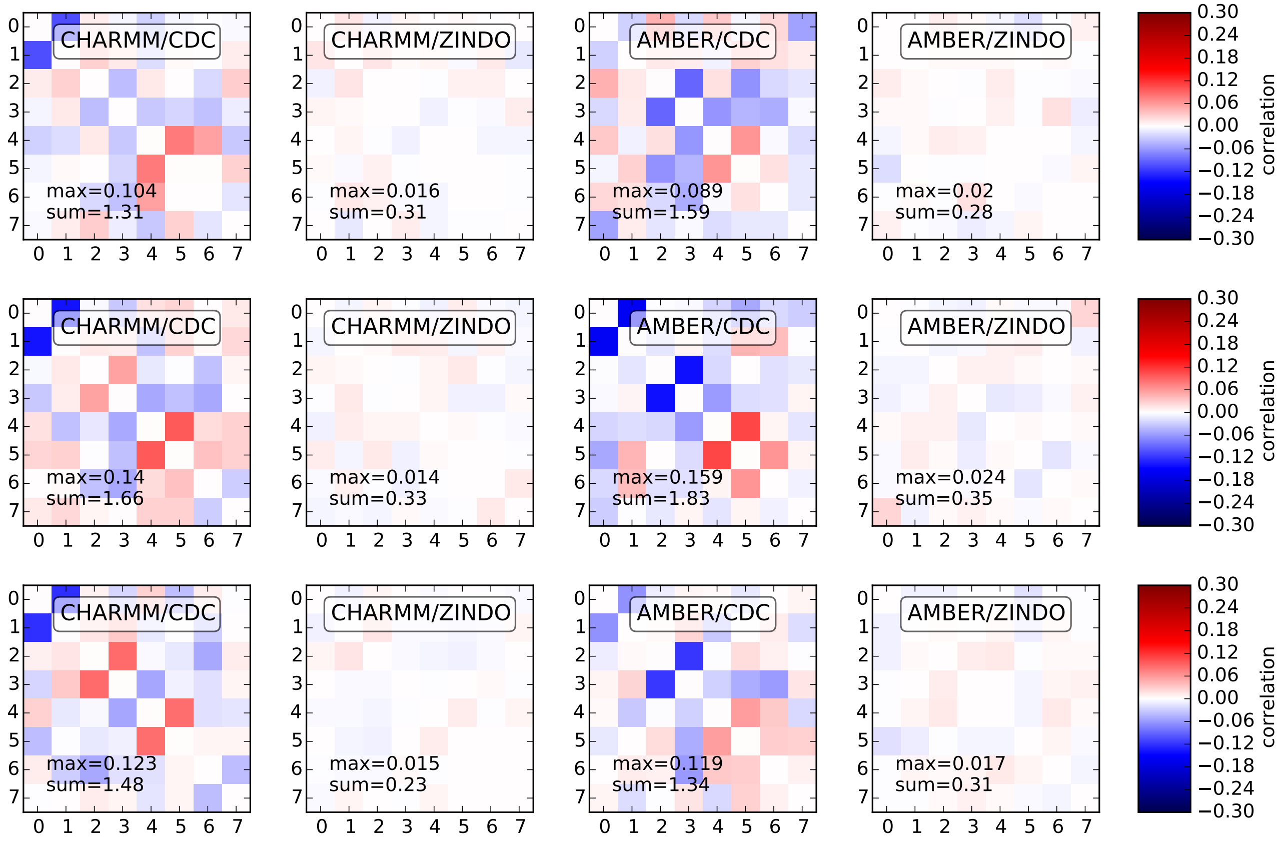


FIG. 6: Same as Fig. 5 but for 77K.

## V. SPECTRAL DENSITIES

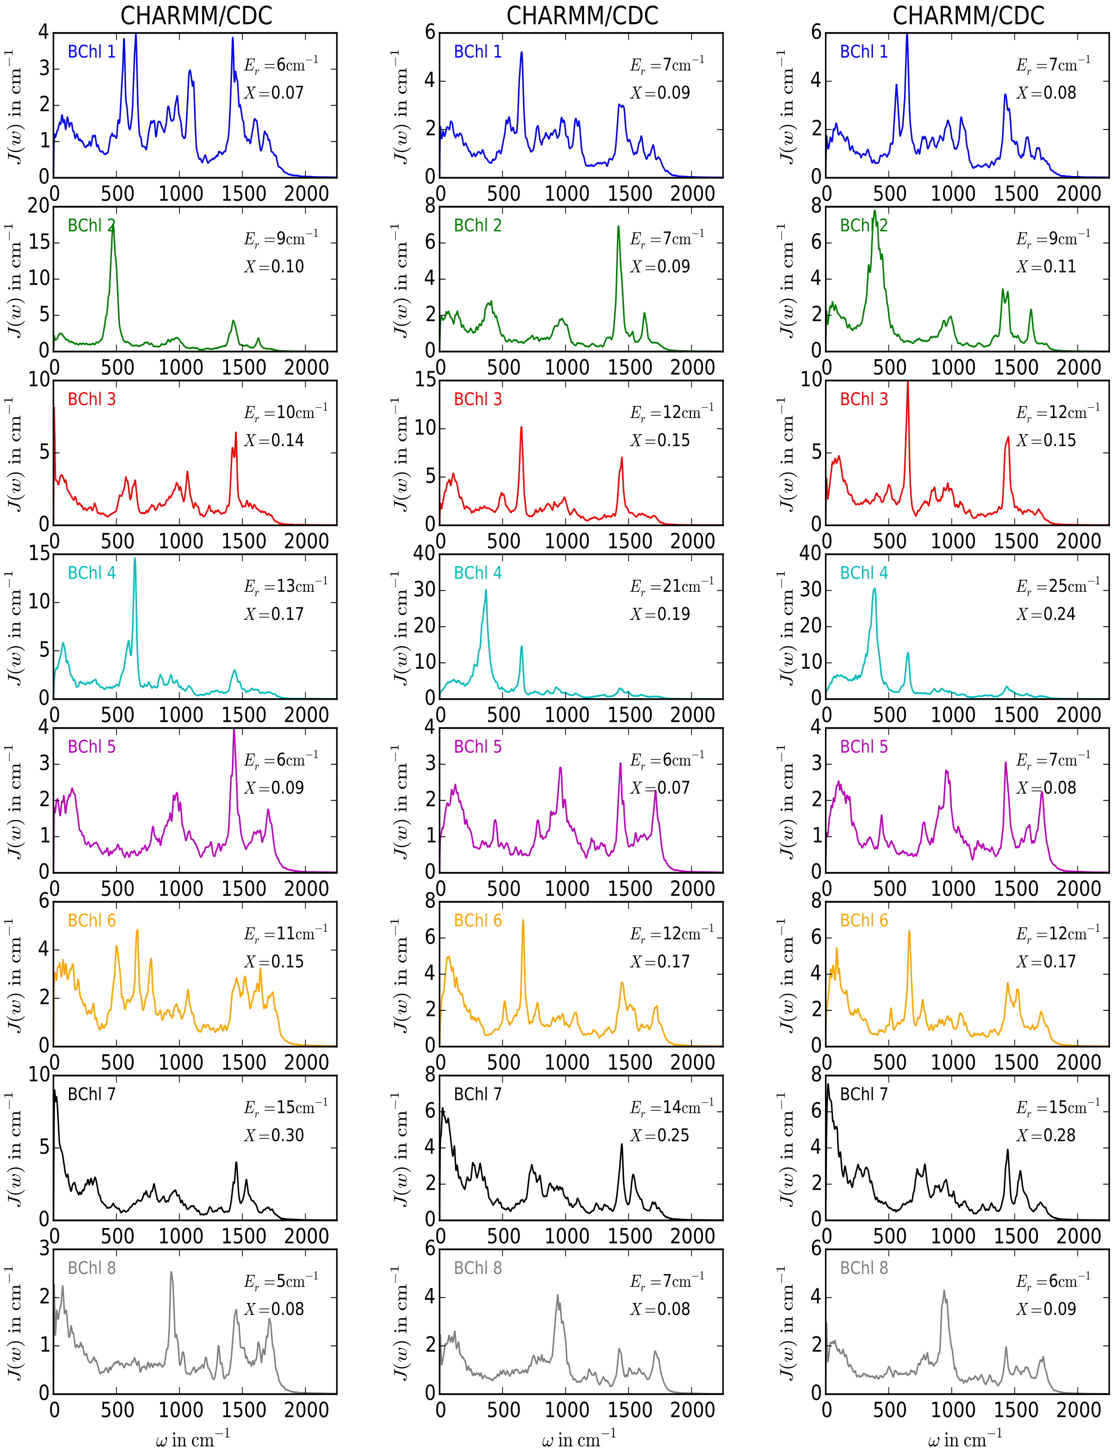


FIG. 7: method 1a, 200K.

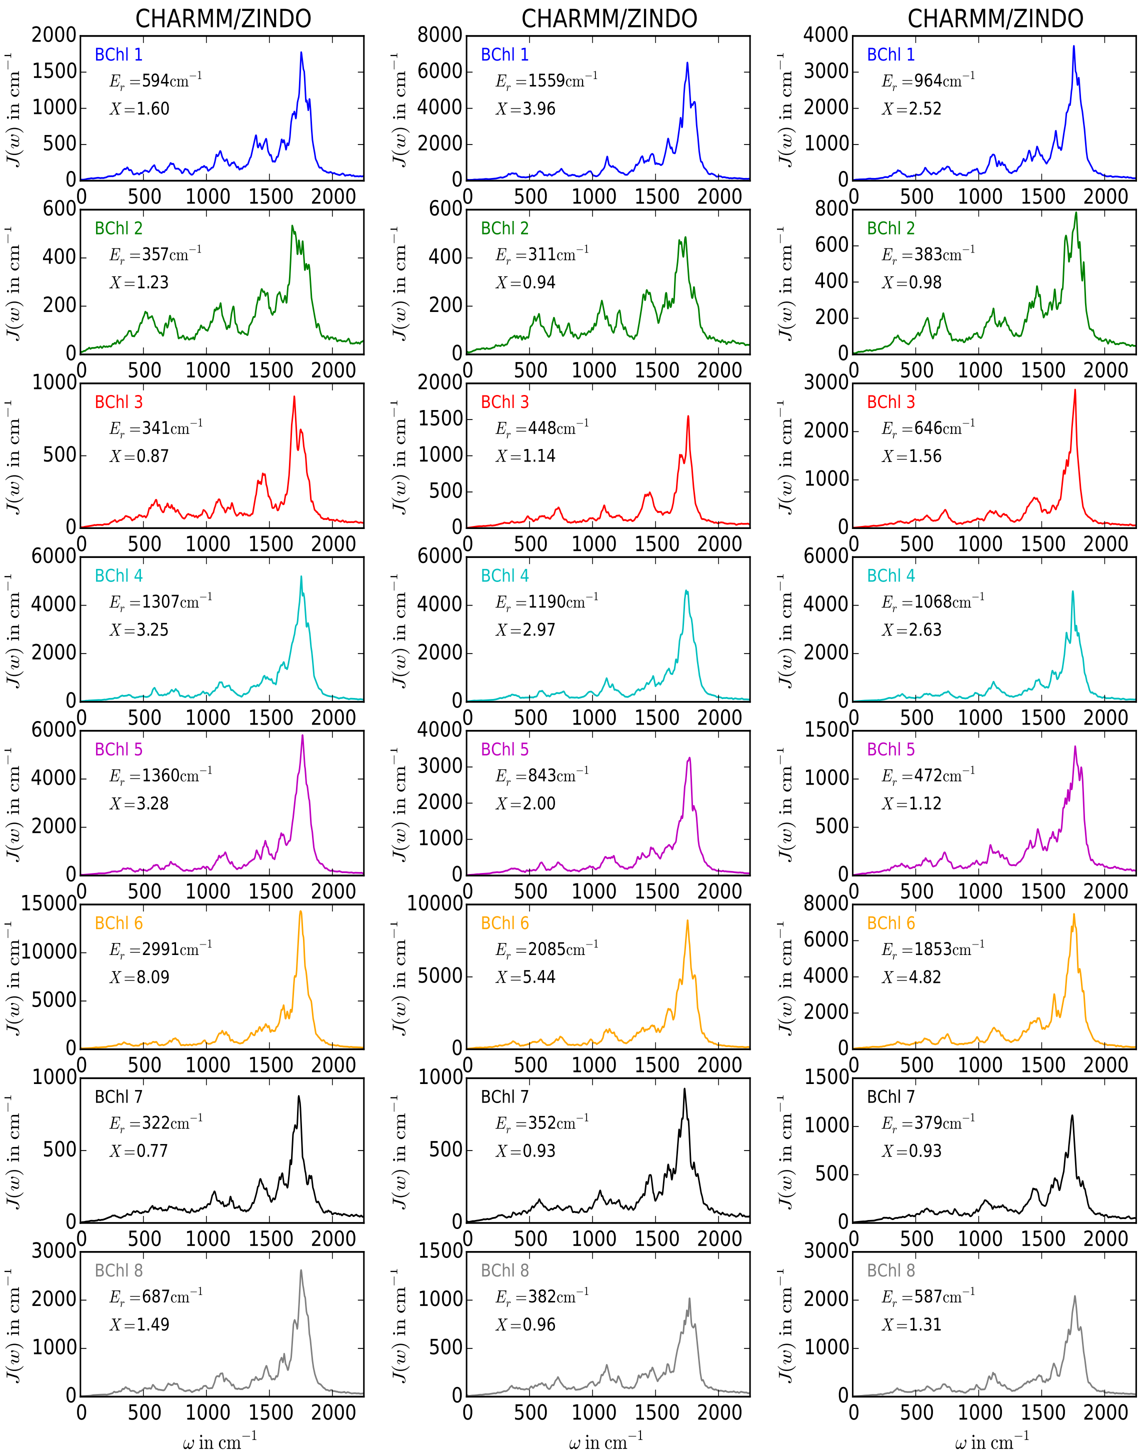


FIG. 8: method 1b, 200K.

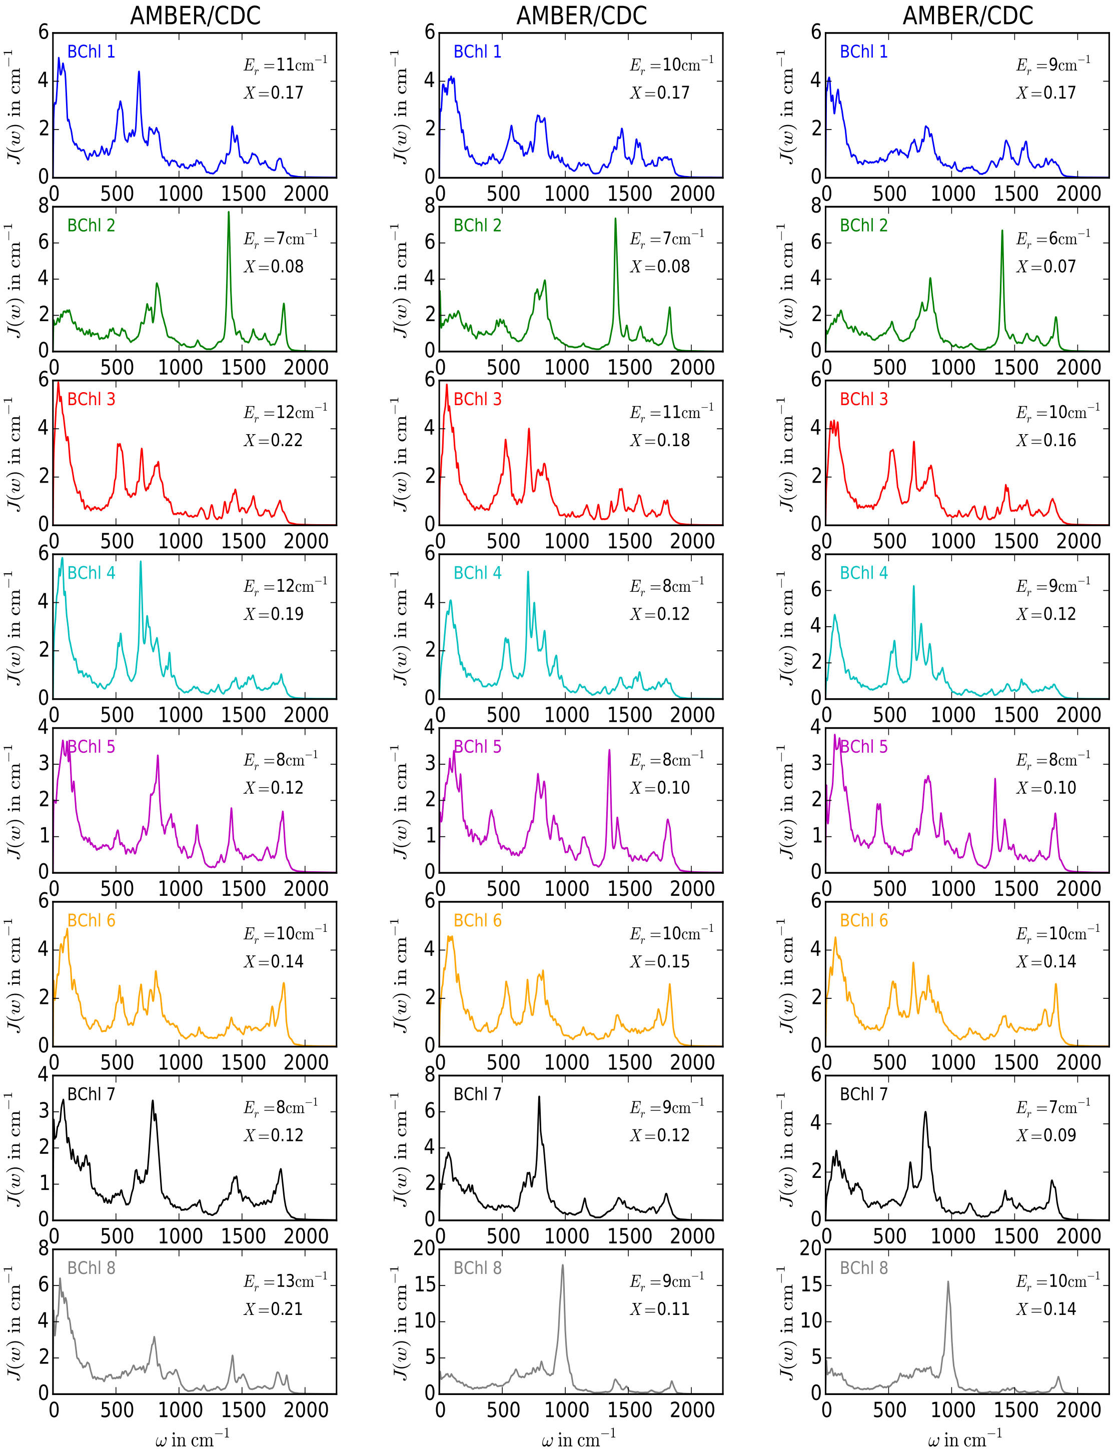


FIG. 9: method 2a, 200K.

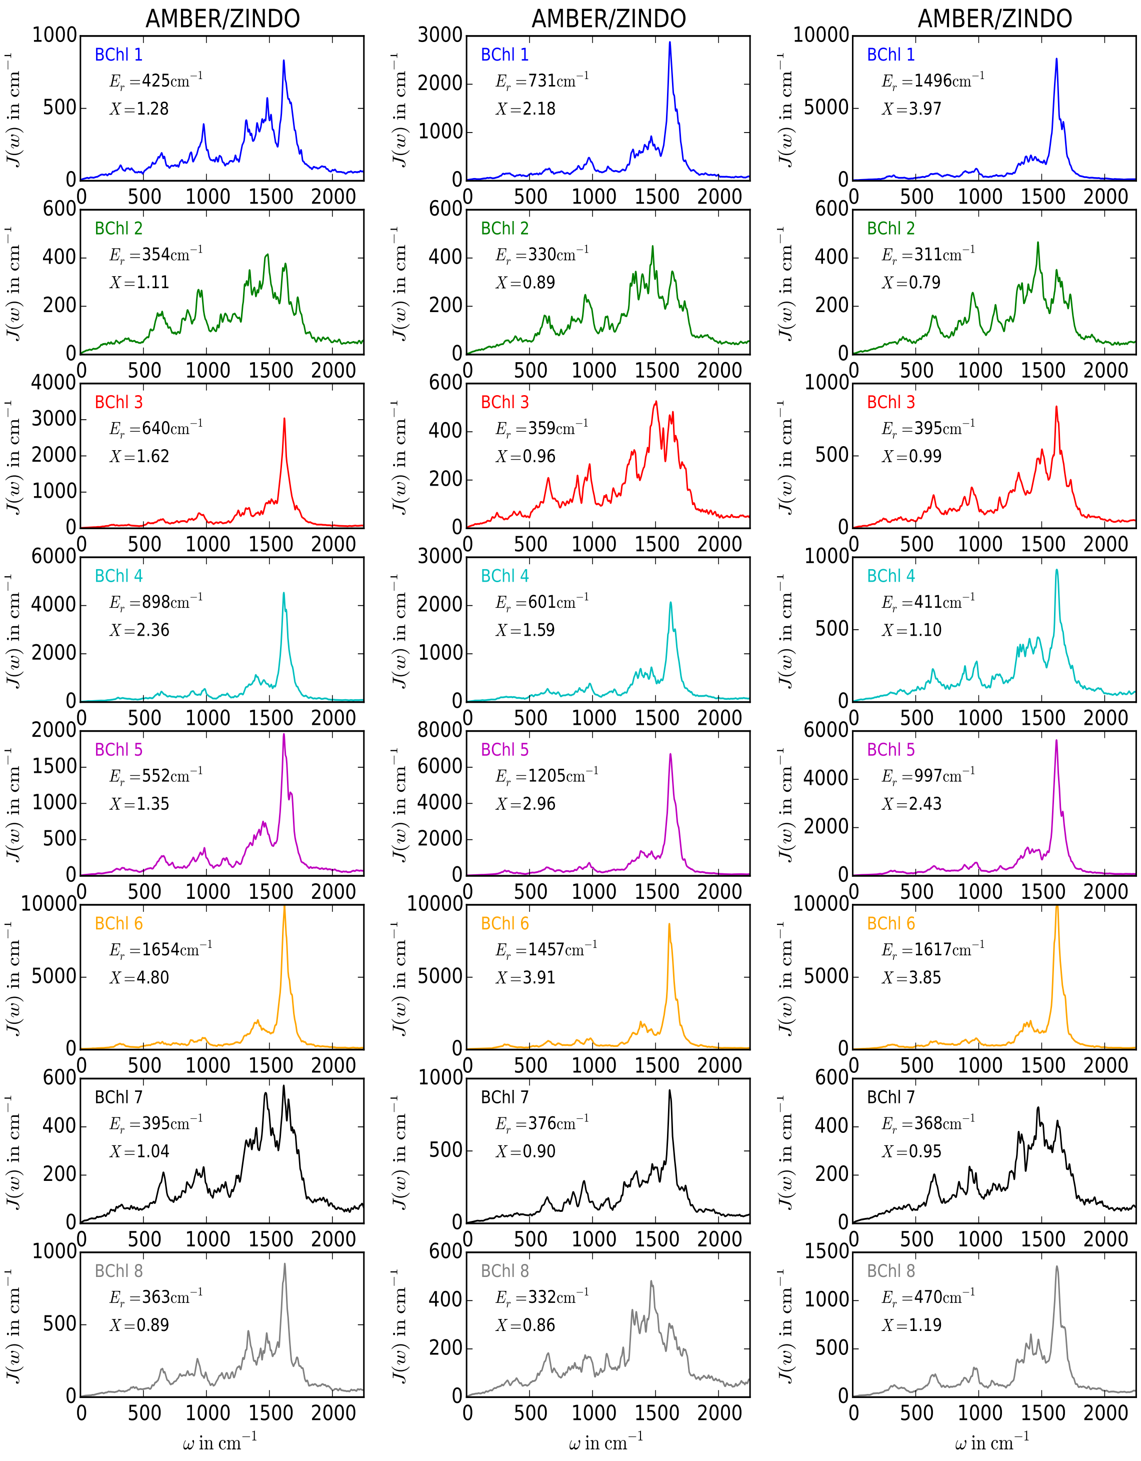


FIG. 10: method 2b, 77K.

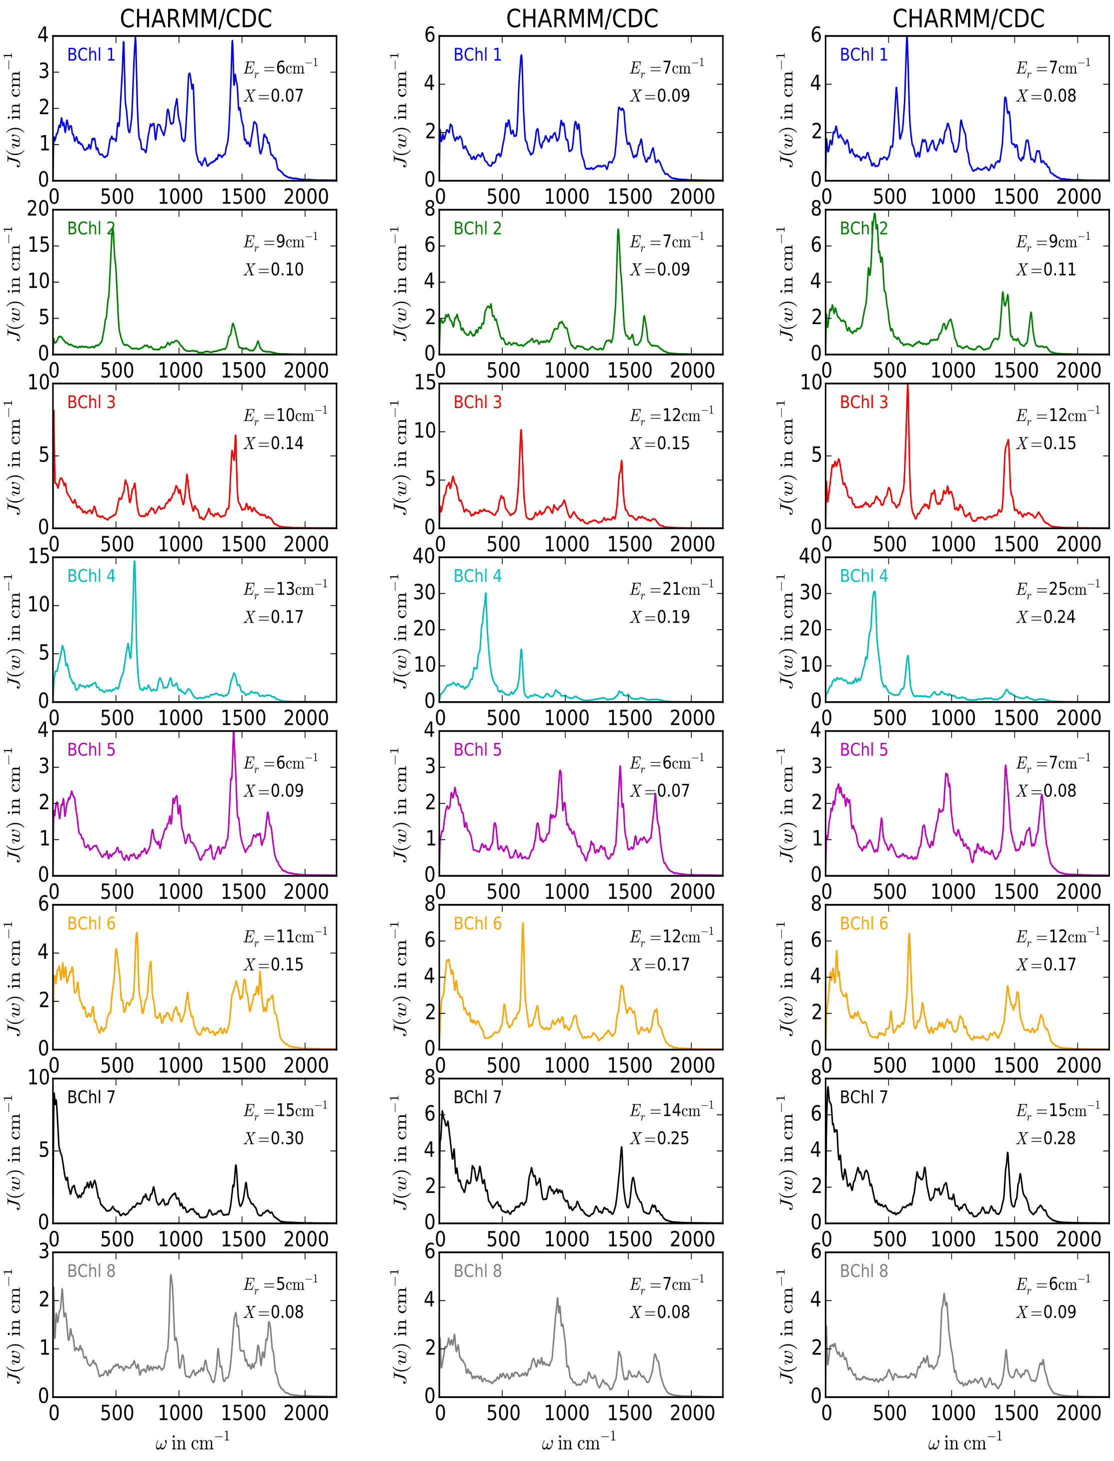


FIG. 11: method 1a, 77K.

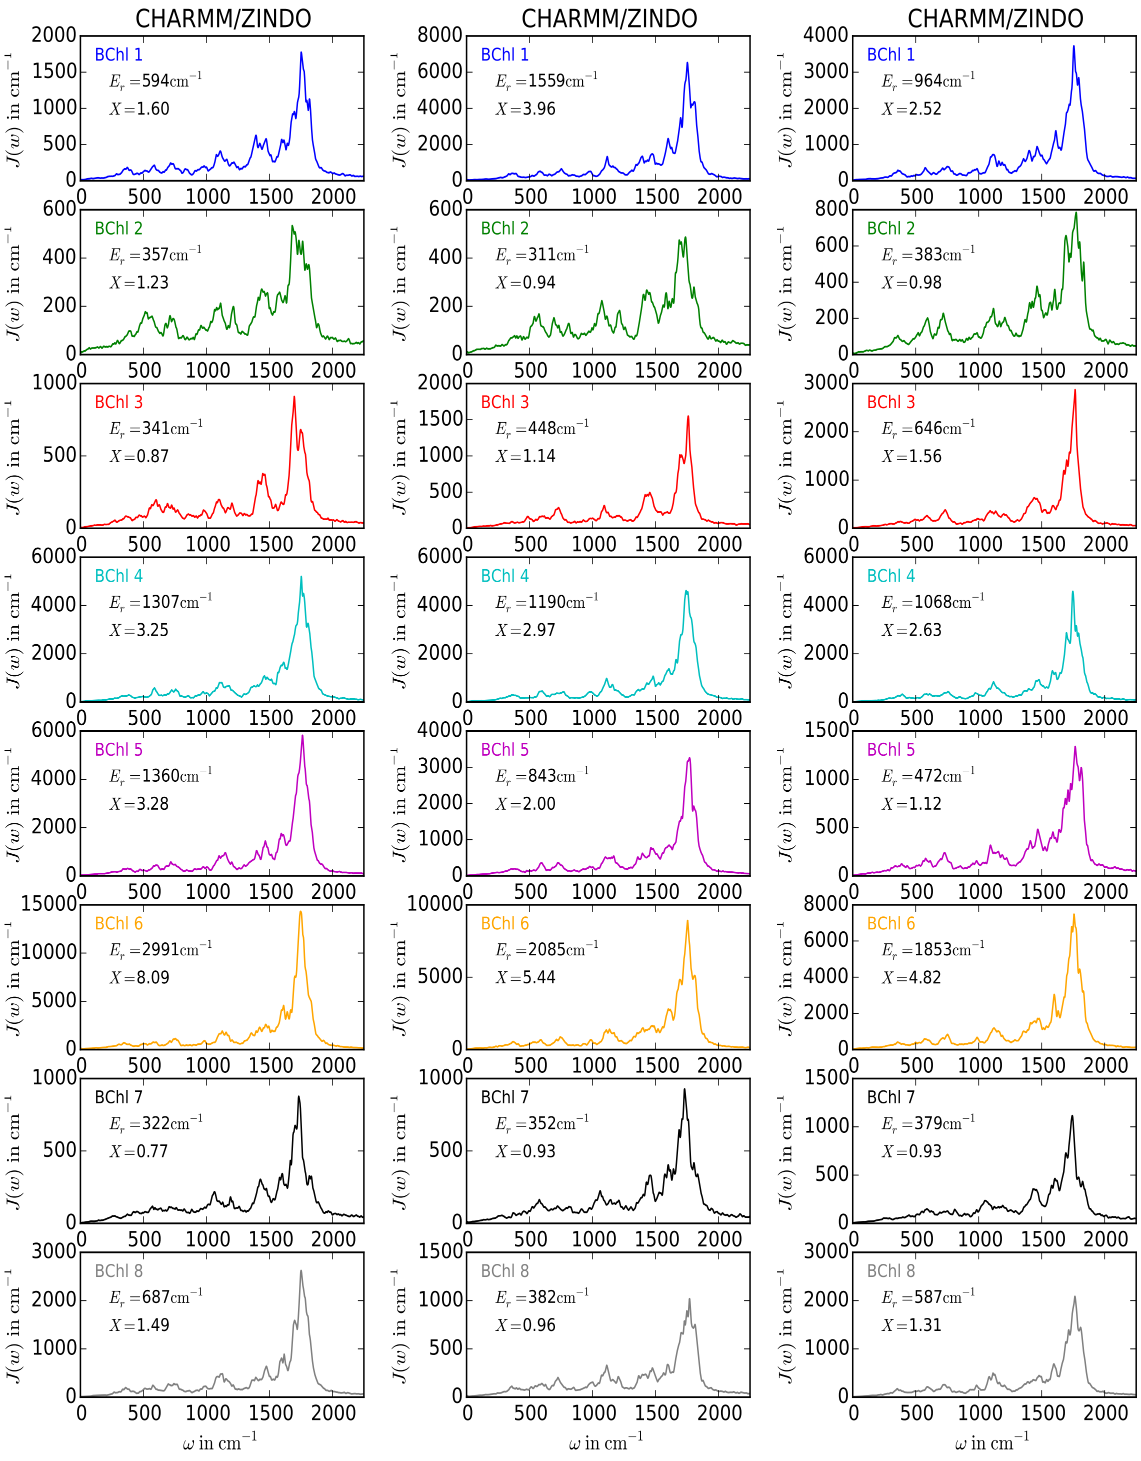


FIG. 12: method 1b, 77K.

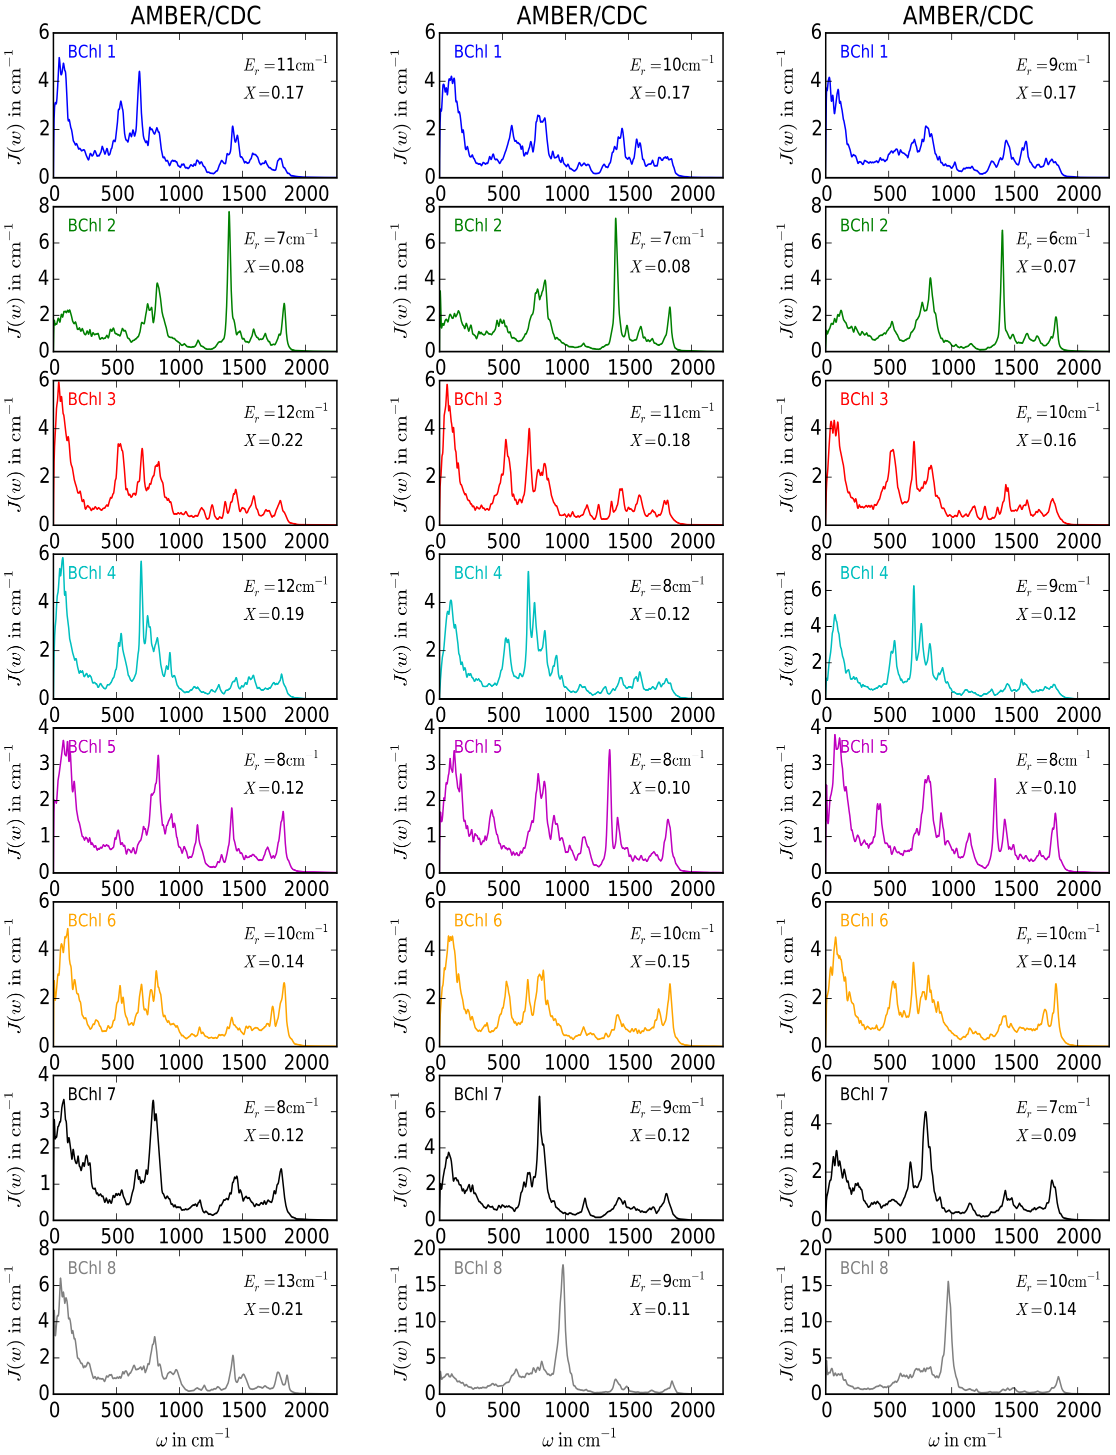


FIG. 13: method 2a, 77K.

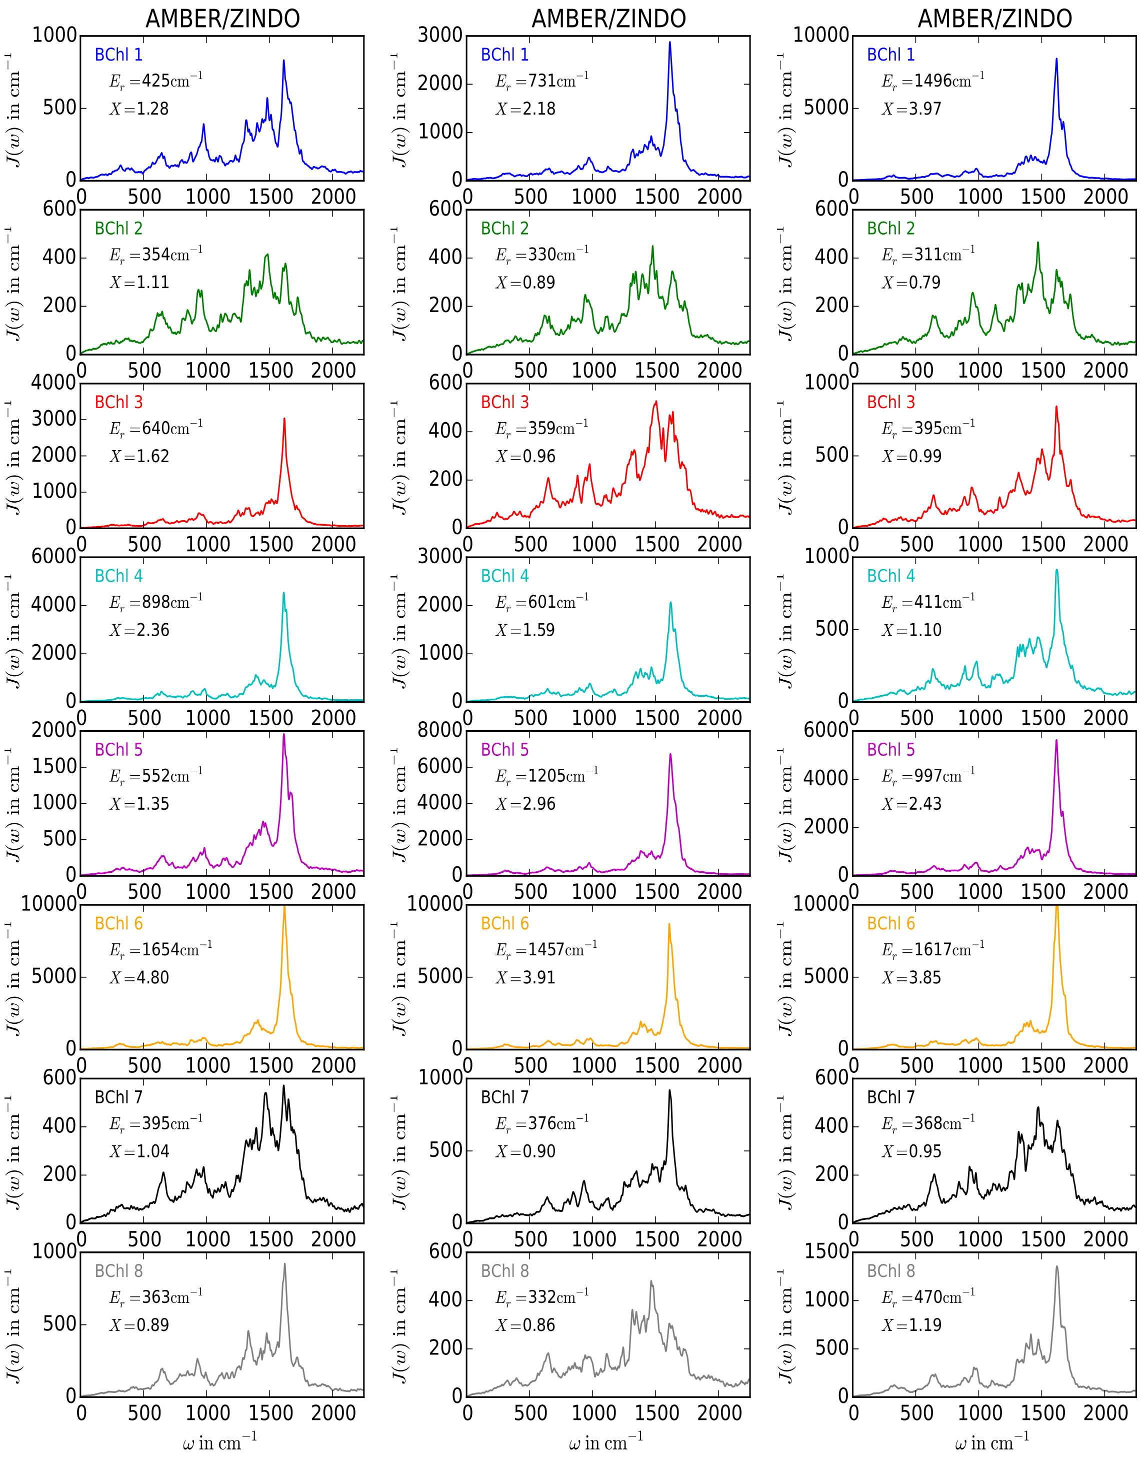


FIG. 14: method 2b, 77K.
